# Supplementary material for: Optimal binary gratings for multi-wavelength magneto-optical traps
Source: arXiv:2306.17080 ancillary file (2023-11-18)
Supplement: Supplementary file 1 [file gMOT_optics_for_Bichromatic_gMOTs__SM_.pdf]

# Optimal binary gratings for multi-wavelength magneto-optical traps – Supplementary material

**Oliver S. Burrow,**[1,*] **Robert J. Fasano,**[2,3] **Wesley Brand,**[2,3] **Michael W. Wright,**[1] **Wenbo Li,**[1] **Andrew D. Ludlow,**[2,3] **Erling Riis,**[1] **Paul F. Griffin,**[1] **and Aidan S. Arnold**[1,†]

[1] *Department of Physics, SUPA, University of Strathclyde, Glasgow, G4 0NG, United Kingdom*
[2] *National Institute of Standards and Technology, 325 Broadway, Boulder, Colorado 80305, USA*
[3] *University of Colorado, Department of Physics, Boulder, Colorado 80309, USA*
[*] *oliver.burrow@strath.ac.uk*
[†] *aidan.arnold@strath.ac.uk*
*https://eqop.phys.strath.ac.uk/atom-optics/grating-mots*

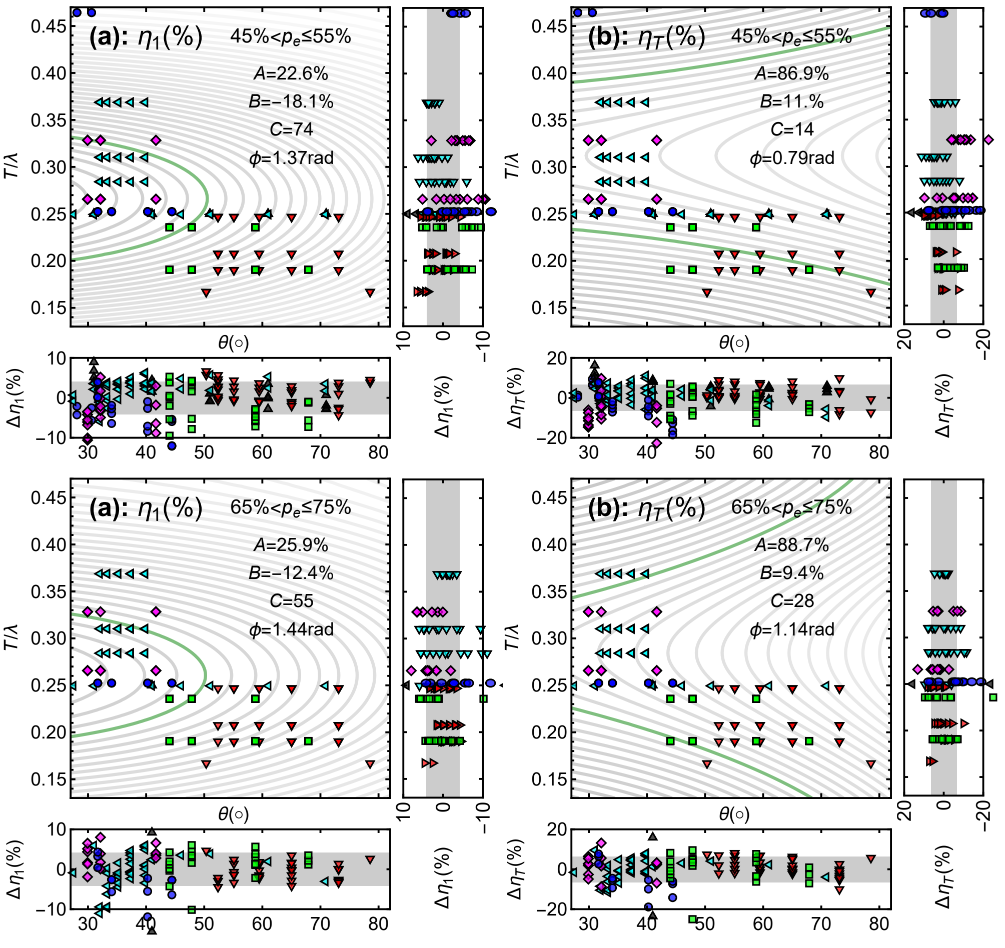


Fig. S1. This figure is the equivalant of Fig. 2 in the main paper, but instead illustrates $\eta_1$ and $\eta_t$ with grating etch duty ranges $45\% < p_e \leq 55\%$ (upper row) and $65\% < p_e \leq 75\%$ (lower row).

To explore how variation of the empirical fit may be a function of the finite range of duty cycles in the fit, we have also investigated duty ranges of 5%, halving the ranges we used in the paper. This leads to the empirical surface fit parameters in Table S1.

| $p_e$ | $A_1$ | $B_1$ | $C_1$ | $\phi_1$ | $\Delta\eta_1$ | $A_t$ | $B_t$ | $C_t$ | $\phi_t$ | $\Delta\eta_T$ |
|---|---|---|---|---|---|---|---|---|---|---|
| 50 | 22.6 | -18.1 | 74 | 1.37 | 4.1 | 86.9 | 11.6 | 14 | 0.79 | 6.6 |
| 60 | 23.2 | -18.7 | 58 | 1.41 | 3.2 | 89.2 | 8.2 | 27 | 0.91 | 5.6 |
| 70 | 25.9 | -12.4 | 55 | 1.44 | 4.2 | 88.7 | 9.4 | 28 | 1.14 | 6.5 |
| 47.5 | 21.2 | -19.0 | 82 | 1.36 | 4.4 | 85.2 | 11.4 | 5.0 | 0.80 | 7.1 |
| 52.5 | 26.5 | -14.4 | 66 | 1.37 | 3.1 | 90.6 | 12.3 | 27 | 0.82 | 5.6 |
| 57.5 | 23.0 | -20.3 | 65 | 1.43 | 3.1 | 90.4 | 8.4 | 31 | 0.73 | 5.5 |
| 62.5 | 26.7 | -13.2 | 52 | 1.38 | 2.9 | 89.0 | 9.8 | 22 | 1.16 | 5.5 |
| 67.5 | 25.1 | -14.1 | 50 | 1.39 | 3.7 | 88.8 | 7.5 | 30 | 0.99 | 5.3 |
| 72.5 | 26.7 | -11.1 | 61 | 1.51 | 4.4 | 89.1 | 11.4 | 28 | 1.18 | 7.1 |

Table S1. The fitted surfaces for $\eta_1$ (left, subscript 1) and $\eta_t$ (right, subscript t), with corresponding RMS fit errors $\Delta\eta_1$, $\Delta\eta_t$. All units are the same as Table 2 in the paper. The $p_e$ values given are the centre of the: ±5% etch duty range (first three rows, duplicating the values in Table 1 of the paper for comparison); ±2.5% etch duty range (last six rows). The number of laser-grating combinations used for the fits in the last six lines of the table were 94, 80, 117, 86, 57, and 67, respectively.

The fit to $\eta_0$ directly using Eq. 1 in the paper led to a slightly worse RMS error to experiment than inferring the value from the two other fits via $\eta_0 = \eta_t - 2\eta_1$. We note this discrepancy can be removed by adding an extra term to the fit function:

$$\eta_i = (1 - C_i\,\theta^2)(A_i + B_i \sin(\phi_i + 4\pi T/\lambda) - \zeta T/\lambda), \tag{S1}$$

where $\zeta$ is a positive dimensionless parameter approximately describing a drop in diffraction efficiency with etch depth. The fit residues for $\eta_1$ and $\eta_t$ in Table S1 barely decrease ($\approx 0.1\%$ change) if the enhanced fit function of Eq. S1 is used. However, both the inferred and particularly the direct $\eta_0$ fit residues are improved and then differ by only $\approx 0.3\%$ – although the inferred $\eta_0 = \eta_t - 2\eta_1$ still has the lowest residue of $3\% < \Delta\eta_0 < 5\%$.

In the remainder of this Supplement we check for any possible remaining trends in the fit residues, but find no strong correlations. We ensure there is no strong variation with laser wavelength, grating diffraction angle or dimensionless grating etch depth, as illustrated in Figs. S2-S4, respectively. Each plot has 6 rows corresponding to the 5% etch duty ranges in Table S1, with the left, middle and right columns show the residues of $\eta_t$, $\eta_1$, and inferred $\eta_0 = \eta_t - 2\eta_1$.

We have also determined how much variance there is in diffraction efficiency for the 'same grating' in terms of all three dimensionless grating parameters of etch duty, diffraction angle and etch depth parameters with binning ranges of 5%, 4°, and 2.5% respectively. This yields RMS variations in $\eta_t$, $\eta_1$, and inferred $\eta_0$ of approximately 3.6%, 2.3% and 2.6%, respectively. We suspect this variation is largely due to the optical characterisation, as we have been informed that: periods are reproducible to 1 nm, etch depths are ±10 nm from target to attained, and the actual duty cycle is checked by scanning electron microscopy.

As a final point of reference, the diffracted circular polarisation purity was measured for most gratings, but this is incomplete and therefore omitted from the dataset. However, the modal and mean average value is good i.e. 90% for the ~400 gratings we have polarisation data for.

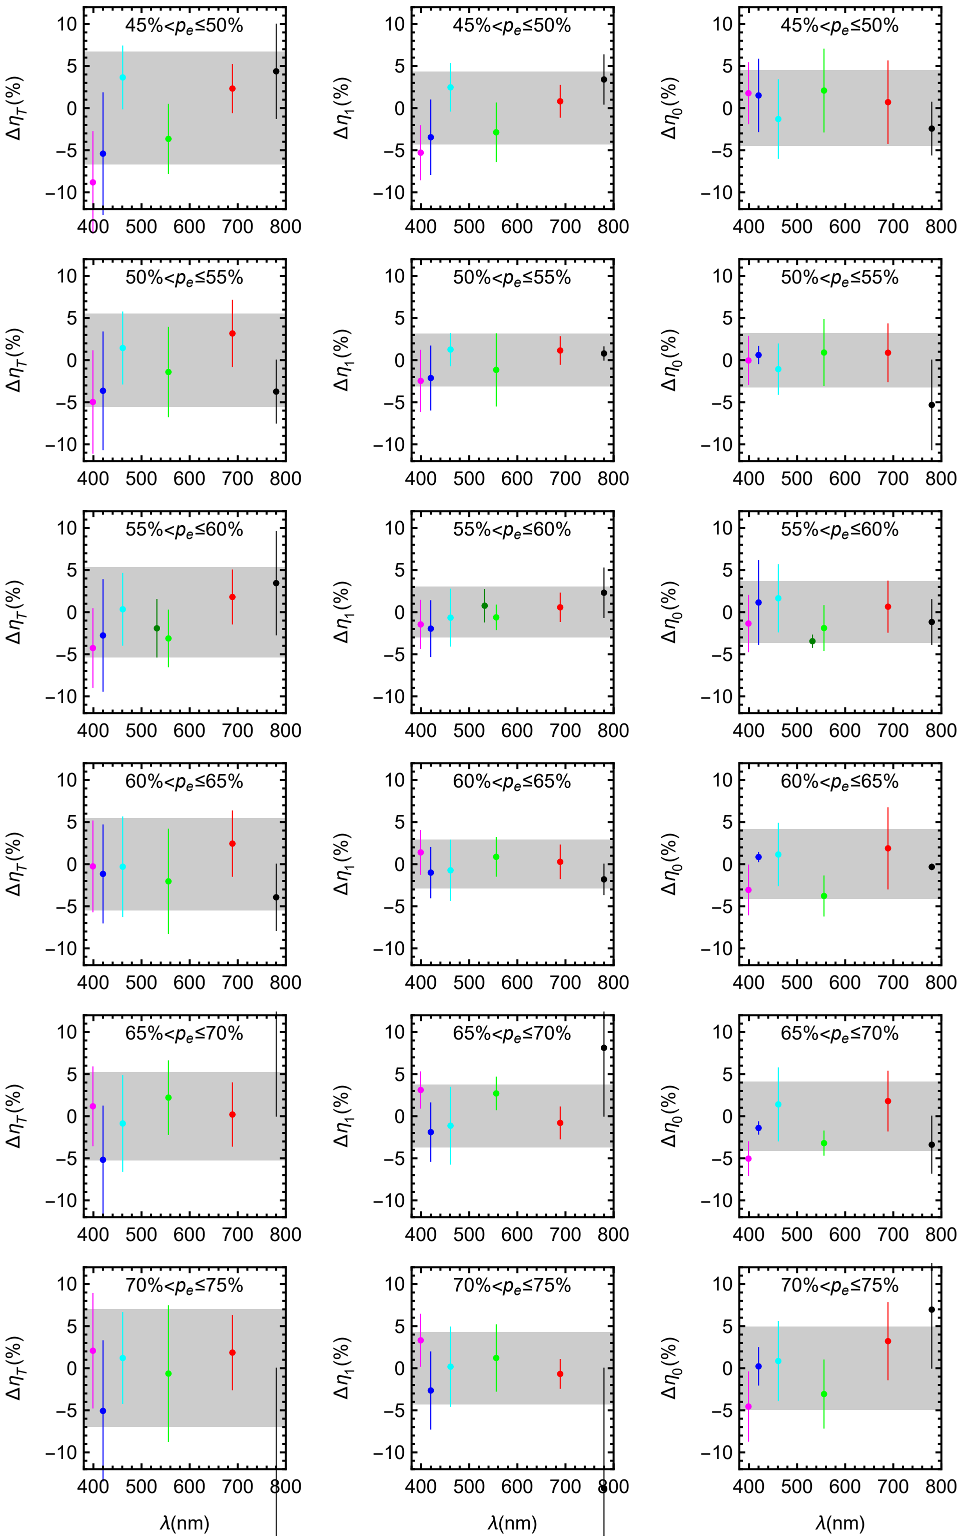


Fig. S2. Fit residuals as a function of testing laser wavelength.

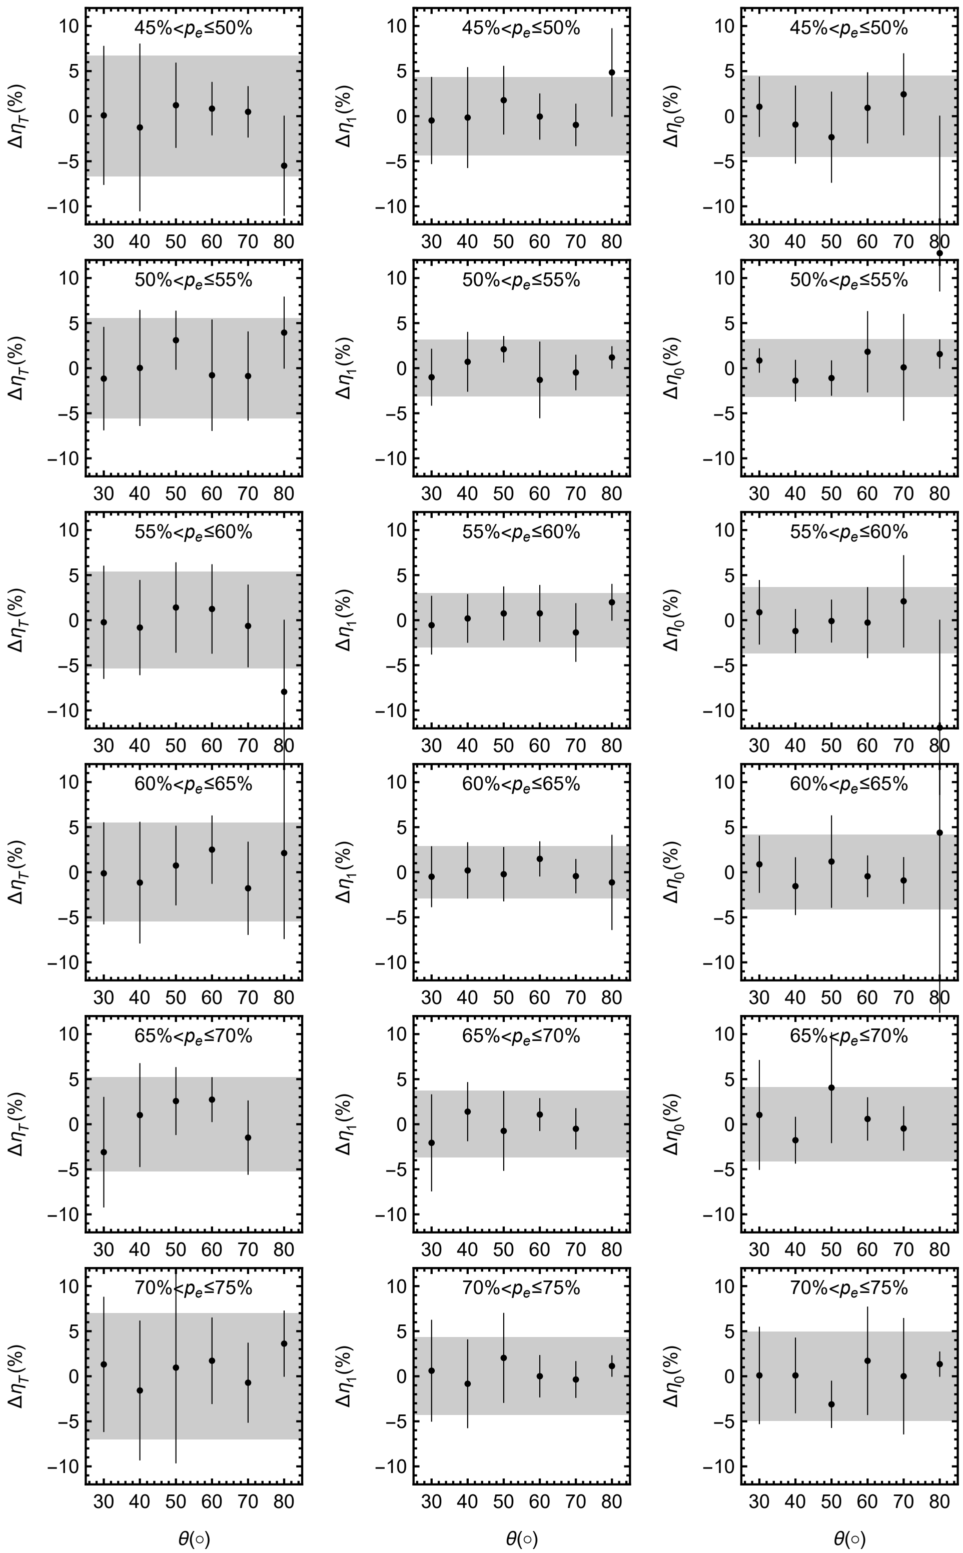


Fig. S3. Fit residuals as a function of grating diffraction angle (i.e. $\theta = \arcsin(\lambda/d)$).

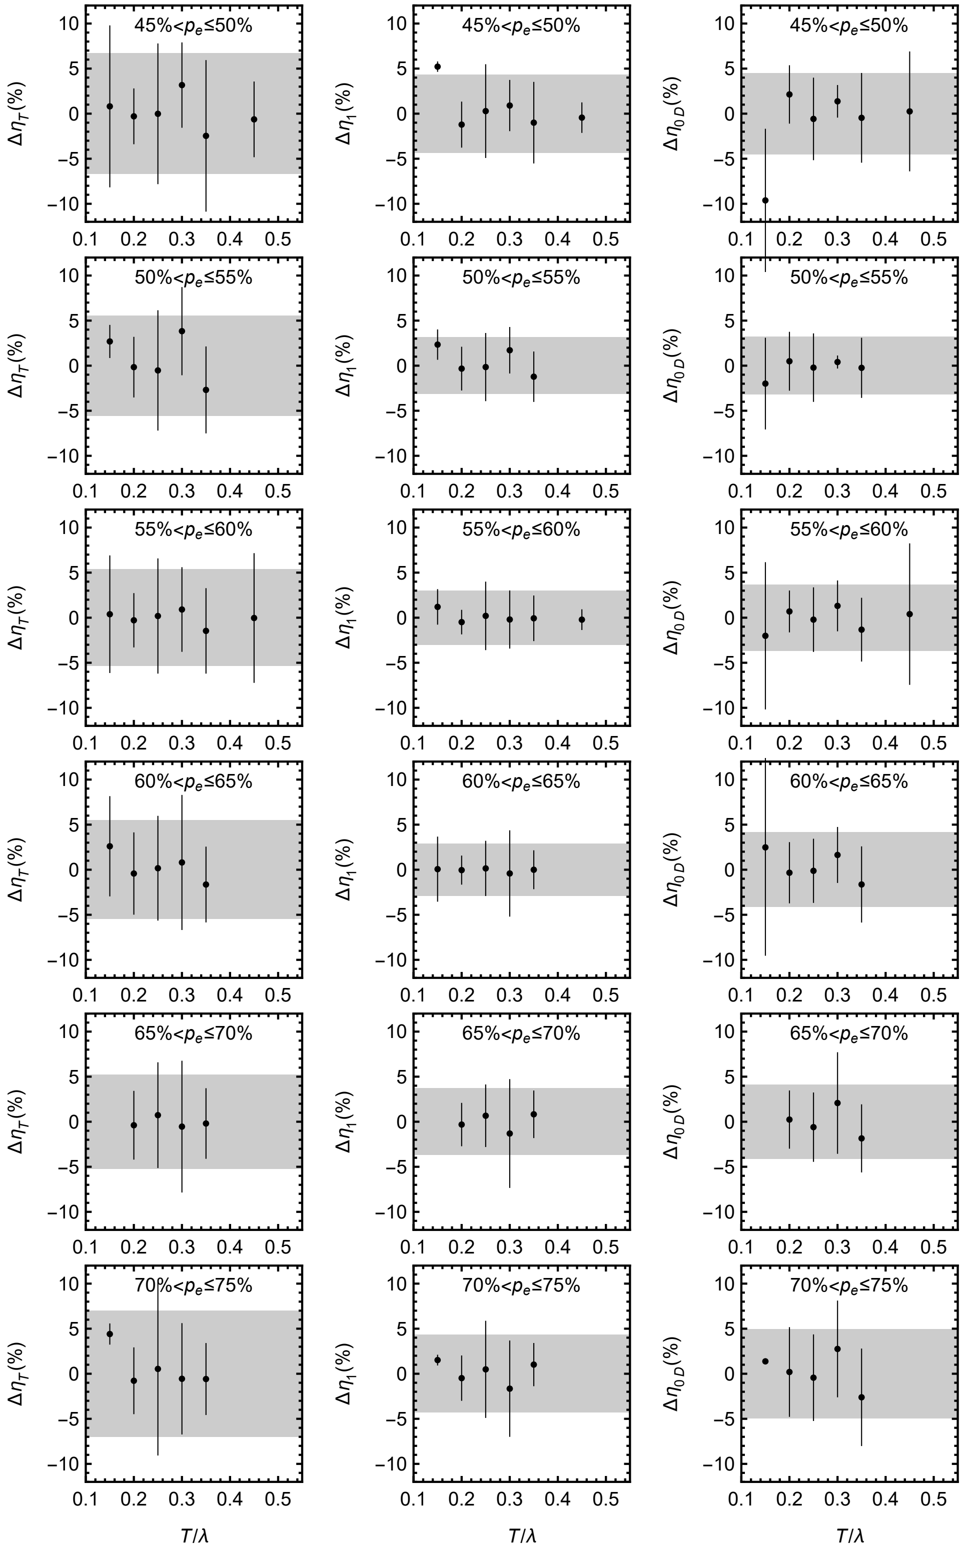


Fig. S4. Fit residuals as a function of dimensionless grating etch depth $T/\lambda$.
